# Supplementary material for: Undirected Graphs of Entanglement Two
Source: arXiv:0705.0419 source file (2007-08-30)
Supplement: Supplementary file 1 [file appendix.tex]

\section{Appendix: proofs for the use of the referee}

\subsection{Decomposition of Graphs in $\zeta_{2}$}
\begin{lemma}[i.e. Lemma \ref{lemma:induct1}]
  Let $G$ be an undirected graph satisfying
  \eqref{cond:no3colls} and \eqref{cond:noadjcolls}.  If $G =
  \theta_{v,b}^{\varepsilon,n} \collapse{b} H$ and $H \in \zeta_2$,
  then there is a subset $\glue' \subseteq V_{G}$ such that
  $(H,\glue')$ is a glue graph in $\zeta_{2}$, $b \in Gl'$, and
  moreover $G$ is the result of the legal collapse
  \begin{align*}
    G & = \theta_{v,b}^{\varepsilon,n} \lcollapse{b} (H,Gl)\,. 
  \end{align*}
  Consequently, $G \in \zeta_2$, with $v$ a glue point of $G$.
\end{lemma}
\begin{proof}
  Since  the graph $H$ is in $\zeta_{2}$, it already comes with a set
  of glue points $\glue_{H}$. Hence, if
  $b \in \glue_H$ then we simply let $\glue' =\glue_H$.
  
  Otherwise $b$ is a dead point of a certain molecule
  $\theta_{c,d}^{\delta,m}$ of $H$, so that we can write
  \begin{align}
    \label{eq:H}
    H & %= \theta_{c,d}^{\delta,m} \lcollapse{d} H'
    = H_{c} \lcollapse{c} \theta_{c,d}^{\delta,m} \lcollapse{d}
    H_{d}\,.
  \end{align}
  Observe also that $m \geq 1$ since $b$ is a dead point of the
  molecule $\theta_{c,d}^{\delta,m}$.

  If $\theta_{v,b}^{\varepsilon,n}$ is disconnected, i.e.
  if $\varepsilon = n = 0$, then the result is obvious, since then
  \begin{align*}
    \theta_{v,b}^{\varepsilon,n} \collapse{b} \theta_{c,d}^{\delta,m}
    \lcollapse{c} H_{c} \lcollapse{d} H_{c}
    & = \theta_{v,b}^{\varepsilon,n}
    \lcollapse[b]{b,c} \theta_{c,d}^{\delta,m}
    \lcollapse{c} H_{c} \lcollapse{d} H_{c} \,.
  \end{align*}
  
  Otherwise, if $\varepsilon + n > 0$, then $\deg[G]{b} \geq 3$, since
  $b$ has two neighbors in the molecule $\theta_{c,d}^{\delta,m}$ and
  at least one neighbor in the molecule
  $\theta_{v,b}^{\varepsilon,n}$.
  
  If $\delta = 0$ then $1 \leq m \leq 2$: condition
  \eqref{cond:noadjcolls} implies that if $m \geq 2$ then $\deg[G]{c}
  = \deg[G]{d} = 2$.  If $m = 1$, then we can use the equality
  \begin{align*}
    \theta^{0,1}_{c,d} & =
    \theta^{1,0}_{c,b} \lcollapse{b} \theta^{1,0}_{b,d}
  \end{align*}
  to add $b$ to the set of glue points of $H$.  If $m = 2$, then
  $\deg[G]{c} = \deg[G]{d} = 2$. Let $e$ be the unique dead point of
  $\theta_{c,d}^{\delta,m} = \theta_{c,d}^{0,2}$ which is distinct
  from $b$. We claim that we can replace the pair $c,d$ with
  $b,e$ in the set of glue points of $H$. As a matter of fact,
  in the algebraic expression \eqref{eq:H} the legal collapses are
  disjoint. This means that we can write
  \begin{align*}
    H_{c} & = H_{c'} \lcollapse{c'} \theta^{0,0}_{c',c} & H_{d} & =
    \theta^{0,0}_{d,d'} \lcollapse{d'} H_{d'} \,,
  \end{align*}
  and consequently we can also write
  \begin{align*}
    H &  = H_{c}
    \lcollapse{c} \theta_{c,d}^{\delta,m}
    \lcollapse{d} H_{d} \\
    & = H_{c'} \lcollapse{c'} \theta^{0,0}_{c',c}
    \lcollapse{c} \theta_{c,d}^{\delta,m}
    \lcollapse{d} 
    \theta^{0,0}_{d,d'} \collapse{d'} H_{d'}
    \\
    & = H_{c'} \lcollapse{c'} \theta^{0,0}_{c',b}
    \lcollapse{b} \theta_{b,e}^{\delta,m}
    \lcollapse{d} 
    \theta^{0,0}_{e,d'} \lcollapse{d'} H_{d'}
    \,.
  \end{align*}
%   where $e$ is the second dead point of the molecule $\theta^{c,d}$.
%   That is, we can replace $c,d$ with $b,e$ in the set of glue points of
%   $H$.

  If $\delta = 1$, then $m = 1$, since condition \eqref{cond:no3colls}
  implies either $\deg{c} = 2$ or $\deg{d} = 2$, hence $m = 1$. Let us
  suppose that $\deg{d} = 2$.  We claim that we can replace $d$ with
  $b$ in the set of glue points of $H$.

  In the algebraic
  expression \eqref{eq:H} the legal collapses on $d$ are disjoint:
  that is we can write
  \begin{align*}
    H_{d} & = \theta^{0,0}_{d,d'} \lcollapse{d'} H_{d'} \,.
  \end{align*}
  Consequently we can write
  \begin{align*}
    H &  = H_{c}
    \lcollapse{c} \theta_{c,d}^{\delta,m}
    \lcollapse{d} H_{d} \\
    & = H_{c}
    \lcollapse{c} \theta_{c,d}^{\delta,m}
    \lcollapse{d} 
    \theta^{0,0}_{d,d'} \lcollapse{d'} H_{d'}
    \\
    & = H_{c} 
    \lcollapse{c} \theta_{c,b}^{\delta,m}
    \lcollapse{d} 
    \theta^{0,0}_{b,d'} \lcollapse{d'} H_{d'}
    \,.
  \end{align*}
  \qed
%   That is, we can replace $d$ with $b$ in the set of glue points of
%   $H$.
\end{proof}

%%% Local Variables: 
%%% mode: latex
%%% TeX-master: "main"
%%% End: 

\subsection{Graphs Without  Long Cycles are Sparse}

Let us recall that a pointed digraph $\langle V,E,v_{0} \rangle$ is a
tree if for each $v \in V$ there exists a unique path from $v_{0}$ to
$v$.
\begin{definition}
  A tree with back-edges is a tuple $\langle V,T,v_{0},B \rangle$ such
  $\langle V,T,v_{0} \rangle$ is a tree, and $B \subseteq V \times V$
  is such that if $x B y$ then $y$ is an ancestor of $x$ in the tree 
  $\langle V,T,v_{0} \rangle$.
\end{definition} 
For a tree with back edge as above let $\delta(v)$ be the length of
the unique path from $v_{0}$ to $v$ on the tree. If $(d,a) \in B$ is a
back edge, then we define
\begin{align*}
  \ell(d,a) & = \delta(d) - \delta(a) + 1\,.
\end{align*}
We observe that $\ell(d,a)$ is the number of vertices on the path from
$a$ to $d$.
\begin{definition}
  A TwBE representation of an undirected connected graph $G = \langle
  V,E\rangle$ is a tree with back edges of the form $\langle
  V,T,v_{0},B \rangle$, satisfying the following conditions:
  \begin{enumerate}
  \item if $\couple{a,b} \in E$, then $(a,b) \in T \cup B$ or $(b,a)
    \in T \cup B$,
  \item $(a,b) \in T \cup B$ implies $(b,a) \not\in T \cup B$,
  \item if $(a,b) \in  T \cup B$, then $\couple{a,b} \in E$.
  \end{enumerate}
\end{definition}
% Clearly, a TwBE representation of an undirected graph is such that $T
% \cap B = \emptyset$. Something more is true: if $(d,a) \in B$, then
% $\ell(d,a) \geq 2$. If $\ell(d,a) = 0$ then $d = a$, but it is not the
% case (by Definition) that $\set{d,d} \in E$. If $\ell(d,a) = 1$, then
% $(a,d) \in T$, contradicting condition 1.
Representations of this kind are obtained by running a DFS on an
undirected graph, according to the following standard Lemma (see
\cite[Theorem 23.9]{Algorithms}).
\begin{lemma}
  Let $(V,\bar{E}_\mathcal{T})$ be a DFS tree of an undirected graph
  $(V,E)$. If an edge $\set{a,b} $ is in $E\setminus
  \bar{E}_{\mathcal{T}}$ then either $a$ is an ancestor of $b$, or $a$
  is a descendant of $b$ in $T$.
\end{lemma}

\begin{lemma}
  A $\langle V,T,v_{0},B \rangle$ tree with back edges such that $0 <
  \ell(d,a) \leq k$ for each back edge $(d,a)$ has at most $(k
  +1)\card{V} -1$ egdes. If $\langle V,T,v_{0},B \rangle$ is a TwBE
  representation of an undirected connected graph, then it has at most
  $(k -1)\card{V} -1$.
\end{lemma}
\begin{proof}
  The edges from $T$ are as usual $|V|-1$. Every vertex $d$ can be the
  source of at most $k$ back edges. Hence we obtain
  \begin{align*}
    \card{T \cup B}
     = \card{T} + \card{B}
    & \leq (\card{V}-1) + k\card{V}
    = (k +1)\card{V} -1\,.
  \end{align*}
  If moreover $\langle V,T,v_{0},B \rangle$ is the representation of
  an undirected graph, we cannot have back edges of the form $(d,d)$,
  not back edges of the form $(d,a)$ if $\ell(d,a) = 1$. Therefore
  Every vertex $d$ can be the source of at most $k-2$ back edges. The
  formula follows as before.  \qed
\end{proof}

\begin{lemma}
  Let $\langle V,T,v_{0},B \rangle$ be a TwBE representation of an
  undirected connected graph $G = \langle V,E\rangle$ whose simple
  cycles have length less than $k$. Then  for each backedge $(d,a)$ we
  have $0 < \ell(d,a) \leq k$.
\end{lemma}
\begin{proof}
  Suppose that $k < \ell(d,a)$, then the path from $a$ to $d$ together
  with the edge from $d$ to $a$ form on $G$ an undirected cycle of
  length $\ell(d,a) > k$.  \qed
\end{proof}

%%% Local Variables: 
%%% mode: latex
%%% TeX-master: "main"
%%% End: 

\subsection{Recognizing Molecules}

\begin{lemma}
  If a biconnected component $C$ is the singleton $\set{v}$, then $v$
  is an isolated point of $G$.
\end{lemma}
\begin{proof}
  Indeed, if $\set{v,u} \in E$, then $\set{v,u}$ is a biconnected
  subset of $G$, since every singleton graph is connected.  \qed
\end{proof}

\begin{lemma}
  If $C$ is a biconnected component of a graph $G = (V,E)$ and $v \in
  C$ is not an articulation point of $G$, then $vE \subseteq C$.
\end{lemma}
\begin{proof}
  Let us suppose that $\couple{v,u} \in E$ for some $u \in V \setminus
  C$ and prove that $v$ is an articulation point of $G$.  It is not
  possible that $C = \set{v}$ since $v$ is not isolated. Therefore
  there exists $x \in C$, $x \neq v$. If in $G$ there exists a path
  from $u$ to $x$ which does not visit $v$, then we can extend $C$ to
  a greater biconnected component to which $u$ belongs. Therefore such
  a path does not exists, and $v$ is an articulation point separating
  $u$ from $x$.  \qed
\end{proof}

\begin{lemma}
  Let $G = (V,E)$ be a biconnected graph and $D \subseteq V$ be such
  that $\set{v \in V \mid \deg{v} \neq 2} \subseteq D$.
  Then $G$ is isomorphic to a molecule, with every element of $D$ sent
  by the isomorphism to a
  glue point of the molecule, if and only if either 
  \begin{align}
    \tag{i} \label{eq:fcase}
    & \card{D} = 2 \text{ and }
    V \setminus D \subseteq dE\,, \;d \in D
    \intertext{or}
    \tag{ii}  \label{eq:scase}
    & \card{D} < 2 \text{ and } \card{V} \in \set{3,4}\,.
  \end{align}
\end{lemma}
\begin{proof}
  Let us consider a biconnected molecule $\theta^{\epsilon,n}_{a,b}$
  and observe first that: (a) $\epsilon + n > 0$ since it is connected
  and (b) $(\epsilon,n) \neq (0,1)$ since it is biconnected.  Let $D
  \subseteq \set{a,b}$ be such that $\set{v \in V \mid \deg{v} \neq 2}
  \subseteq D$: clearly $\card{D} \leq 2$.

  If $\card{D} = 2 $, then $D = \set{a,b}$ and \eqref{eq:fcase} holds.
  If $\card{D} < 2$ then $\theta^{\epsilon,n}_{a,b}$ contains at most
  one vertex of degree distinct from $2$. Since $\deg{a} = \deg{b} =
  \epsilon + n$, this implies that $\theta^{\epsilon,n}_{a,b}$
  contains no vertex of degree distinct from $2$. We have therefore
  $(\epsilon,n) = (0,2)$ and $\card{V} = 4$ or $(\epsilon,n) = (1,1)$
  and $\card{V} = 3$ so that \eqref{eq:scase} holds.

  Conversely, let us consider a biconnected graph $G = (V,E)$ and let
  $D \subseteq V$ be such that $\set{v \in V \mid \deg{v} \neq 2}
  \subseteq D$.

  Let us suppose that \eqref{eq:fcase} holds and let $D = \set{a,b}$.
  Therefore if $x \not\in D$, then $\deg{x} = 2$ and since
  $\couple{x,a},\couple{x,b} \in E$, then $\set{a,b} = xE$. We have
  therefore that $G$ is isomorphic to $\theta^{\epsilon,n}_{a,b}$
  where $n = \card{V} -2$ and $\epsilon = 1$ if $\set{a,b} \in E$ and
  otherwise $\epsilon = 0$.

  Let us suppose that \eqref{eq:scase} holds, i.e. that $\card{D} < 2$
  and $\card{V} \in \set{3,4}$. Let us assume first that $\card{V} =
  3$. By looking at the list of graphs with $3$ vertices, we observe
  that only the total graph $K_{3}$ is biconnected, hence $G$ is
  isomorphic to $\theta^{1,1}_{a,b}$.
  If $\card{V} = 4$, then we claim that every vertex of $G$ has degree
  $2$, so that $G$ is isomorphic to $\theta^{0,2}_{a,b}$.  To prove
  the claim, observe that $G$ may have at most one vertex whose degree
  is not $2$. Suppose that such a vertex exists and call it $v_{0}$,
  so that $\deg{v_{0}} \in \set{1,3}$ since $G$ is connected.
  Then the usual formula 
  \begin{align*}
    2\card{E} & = \deg{v_{0}} + \sum_{v \neq v_{0}} \deg{v}
    = \deg{v_{0}} + 6
  \end{align*}
  leads to a contradiction.  \qed
\end{proof}

%%% Local Variables: 
%%% mode: latex
%%% TeX-master: "main"
%%% End: 

%%% Local Variables: 
%%% mode: latex
%%% TeX-master: "main"
%%% End: 
